# Supplementary material for: Semi-Supervised Domain Generalization for Object Detection via Language-Guided Feature Alignment
Source: arXiv:2309.13525 source file (2023-09-24)
Supplement: Supplementary file 1 [file supplement.tex]

% \section{Supplement}

We compare our proposed model against source-only fully-supervised object detection models (FSOD), domain adaptation (DA), and domain generalization (DG) baselines on two benchmarks, \textit{real-to-artistic} and \textit{adverse weather}. Pre-trained ResNet50 by RegionCLIP is utilized as the backbone in this project; therefore, for a fair comparison, we only compare it with related works utilizing the ResNet50 backbone. Note that larger pre-trained ResNet backbones, such as ResNet101, are not yet available for RegionCLIP by the authors \cite{zhong2022regionclip}. 
To our knowledge, DIDN \cite{lin2021domain} is the only multi-domain DG work in object detection, but it only conducted experiments on adverse weather, and its implementation code is not publicly available, preventing fair comparison on \textit{real-to-artistic}. Thus, on the DG task in real-to-artistic transfer, we compare to source-only FSOD baselines (i.e., Faster-RCNN and RegionCLIP), domain adaptation methods, namely Adaptive-MT \cite{he2022cross}, IRG \cite{he2022cross}, and our defined DG baselines, namely \textit{Direct Visual Alignment (DVA)} and \textit{Caption Pseudo-Labeling (Caption-PL)} in Table \ref{tab:DG-voc-supplement} as well as in Table 1 and Table 3.a in the main text. Generally, Table \ref{tab:DG-voc-supplement} is an extension of Table 1 in the main text, containing DVA and Caption-PL results for all settings. We extended our approach to the DA task and compared it with source-only FSOD baselines,  DA methods, and our defined DG baselines on \textit{real-to-artistic} in Table \ref{tab:DA-voc} in this document. We further compare our model on \textit{adverse weather} DG task with source-only FSOD baselines and DIDN \cite{lin2021domain} in Table \ref{tab:DG-city}. Following \cite{lin2021domain}, and since most of the previous works have used these benchmarks in their experiments, we have extensively compared our model on the \textit{City $\rightarrow$ Foggy} adaptation task, against both source-only FSOD and DA baselines. These comparisons can be seen in Table 2 of the main text. SW-DA \cite{saito2019strong}, D\&Match \cite{kim2019diversify}, MTOR \cite{cai2019exploring}, AFAN \cite{wang2021afan}, GPA \cite{xu2020cross}, SFA \cite{wang2021exploring}, DSS \cite{wang2021domain}, TTD+FPN \cite{he2022cross}, and IRG \cite{he2022cross} are the DA sota that are compared with on this task. Finally, we include some qualitative results by comparing the generated caption using ClipCap based on RegionCLIP and our method's visual features in Table \ref{tab:caption-compare}. Table \ref{tab:predictions-compare-voc} and \ref{tab:predictions-compare-city} visualize the inference of our model and RegionCLIP baseline on \textit{real-to-artistic} and \textit{adverse weather} tasks, respectively.

\section{Quantitative results \& experimental settings}
\textbf{Real-to-artistic.} This benchmark includes three settings for both the DG and DA tasks, where the choice of the unlabeled source and target domains can be clipart, watercolor, or comic. In all settings, Faster-RCNN and RegionCLIP are trained on VOC in a supervised manner forming our source-only FSOD baselines. In the DG task, we compare against source-only FSOD baselines and Adaptive-MT and IRG as domain adaptation methods in Table \ref{tab:DG-voc-supplement} and Table 1 in the main text. For a fair comparison, we adopted and trained the Adaptive-MT with a ResNet50 backbone. Note that unsupervised domain adaptation works can be extended to domain generalization and semi-supervised domain generalization tasks as they do not use labels in the target domain. However, as shown in Table \ref{tab:DG-voc-supplement}, our method achieves a superior performance to domain adaption methods. This proves two of our hypotheses: the effectiveness of vision-language pretraining in learning robust and generalized object detectors and the impact of cross-domain descriptive multi-scale learning (CDDMSL). As no DG in object detection work experimented on \textit{real-to-artistic} benchmark, we defined two other DG methods, \textit{Direct Visual Alignment} and \textit{Caption-PL} and compared with our method on different DG settings in Table \ref{tab:DG-voc-supplement} and DA task of \textit{VOC $\rightarrow$ Clipart} in Table 3.a in the main text. Note they both are trained with the same parameters and take advantage of vision-language pretraining (i.e., RegionCLIP), making them a strong baseline. The results show the advantage of CDDMSL compared to enforcing the domain-invariant learning in visual space and token space in both DG and DA settings.

Table \ref{tab:DA-voc} compares our model against source-only baselines, state-of-the-art DA methods, and our own defined DG baselines on this task. Our method achieves superior performance in almost all settings, demonstrating the efficacy of CDDSML in learning semantically robust domain-invariant features. In particular, we enforce the model to learn visual features that enable the \emph{v2l} layer to produce consistent descriptive features across two images with the same semantics but different styles. This enforces the model to learn invariant features while retaining semantically important information crucial for object detection. Although IRG achieves a higher mAP on \textit{VOC $\rightarrow$ Watercolor}, our method significantly outperforms it on \textit{VOC $\rightarrow$ Clipart} and \textit{City $\rightarrow$ Foggy} (Table 2 in the main text). We conjecture that this is because watercolor is the most similar domain to the labeled source domain (i.e., VOC). In fact, we observe on all tasks that both domain adaption methods and source-only FSOD baselines consistently perform better on watercolor compared to the other settings. This shows that watercolor is an easier target.
\begin{table}[!tp]
\scriptsize
\centering
  \captionsetup{skip=0pt, position=above} % Force the caption to be above the table
 \caption{\textbf{Real-to-artistic generalizations (Extended Results)}. Numbers in parentheses show the difference from RegionCLIP. Max $\uparrow$ shows maximum improvement over two target domains compared to F-RCNN. We report mAP ($\%$). $\dagger$/$\ddagger$ denote DA methods/labeled source-only methods.
 %, respectively.
 }
  \label{tab:DG-voc-supplement}
\begin{tabular}{@{\hspace{3pt}}llllllll@{\hspace{1pt}}} 
\toprule
% \grayrow
    \multirow{2}{*}{{Method}}&
    \multicolumn{2}{l}{{VOC\&Clip \textrightarrow Water,Com}}  & 
    \multicolumn{2}{l}{{VOC\&Water\textrightarrow Clip,Com}} &
    \multicolumn{2}{l}{{VOC\&Com\textrightarrow Clip,Water}}&
    \multirow{2}{*}{Max $\uparrow$ }\\  
\cmidrule(lr){2-3}\cmidrule(lr){4-5}\cmidrule{6-7}
& Watercolor&Comic&Clipart&Comic&Clipart&Watercolor&\\
\hline
\multicolumn{1}{l|}{F-RCNN$\ddagger$ \cite{ren2015faster}} &41.2&17.9&24.1&17.9&24.1&41.2&\multicolumn{1}{|l}{-}\\
\multicolumn{1}{l|}{R-CLIP$\ddagger$ \cite{zhong2022regionclip}}  &44.7&34.2&33.9&34.2&33.9&44.7&\multicolumn{1}{|@{\hspace{3pt}}l@{\hspace{3pt}}}{16.3/16.3/9.8}\\
\hline
\multicolumn{1}{l|}{Adaptive MT$\dagger$ \cite{li2022cross}} &40.6 \tiny{\textcolor{red}{(-4.1)}}&22.2 \tiny{\textcolor{red}{(-12.0)}}&29.0 \tiny{\textcolor{red}{(-4.9)}}&24.3 \tiny{\textcolor{red}{(-9.9)}}&25.7 \tiny{\textcolor{red}{(-8.2)}}&42.3 \tiny{\textcolor{red}{(-2.4)}}&\multicolumn{1}{|@{\hspace{3pt}}l@{\hspace{0pt}}}{4.3/6.4/1.6}\\
\multicolumn{1}{l|}{IRG$\dagger$ \cite{vs2022instance}} &48.1 \tiny{\textcolor{blue}{(+3.4)}}&25.9 \tiny{\textcolor{red}{(-8.3)}}&-&-&-&-&\multicolumn{1}{|@{\hspace{3pt}}l@{\hspace{3pt}}}{8.0/-/-}\\
\hline
\multicolumn{1}{l|}{DVA} &45.6 \tiny{\textcolor{blue}{(+0.9)}}&38.1 \tiny{\textcolor{blue}{(+3.9)}}&
32.6 \tiny{\textcolor{red}{(-1.3)}} &34.2 \tiny{\textcolor{blue}{(+0.0)}}&35.9 \tiny{\textcolor{blue}{(+2.0)}}&45.9 \tiny{\textcolor{blue}{(+1.2)}}&\multicolumn{1}{|@{\hspace{3pt}}l@{\hspace{0pt}}}{20.2/-/11.8}\\
\multicolumn{1}{l|}{Caption-PL} &45.0 \tiny{\textcolor{blue}{(+0.3)}}&36.4 \tiny{\textcolor{blue}{(+2.2)}}&30.1 \tiny{\textcolor{red}{(-3.8)}}&30.3 \tiny{\textcolor{red}{(-3.8)}}&34.7 \tiny{\textcolor{blue}{(+0.8)}}&42.1 \tiny{\textcolor{red}{(-2.6)}}&\multicolumn{1}{|@{\hspace{3pt}}l@{\hspace{0pt}}}{18.5/12.4/10.6}\\

\multicolumn{1}{l|}{\textbf{Ours}}  &\textbf{49.8} \tiny{\textcolor{blue}{(+5.1)}}&\textbf{45.9} \tiny{\textcolor{blue}{(+11.7)}}&\textbf{38.7} \tiny{\textcolor{blue}{(+4.8)}}&\textbf{43.5} \tiny{\textcolor{blue}{(+9.3)}}&\textbf{39.8} \tiny{\textcolor{blue}{(+5.9)}}&\textbf{49.4} \tiny{\textcolor{blue}{(+5.2)}}&\multicolumn{1}{|@{\hspace{3pt}}l@{\hspace{3pt}}}{\textbf{28.0}/\textbf{25.6}/\textbf{15.7}}\\
% Target only & && & &\\
\bottomrule
\end{tabular}
\end{table}

\begin{table}[!tp]
\centering
\captionsetup{skip=0pt, position=above} % Force the caption to be above the table
\caption{\textbf{Domain Adaptation on real-to-artistic}. Results are reported in all three settings: (1) VOC $\rightarrow$ Clipart (2) VOC $\rightarrow$ Watercolor (3) VOC $\rightarrow$ Comic}
\label{tab:DA-voc}
\scriptsize
\begin{spreadtab}{{tabular}{l|c@{\hspace{0pt}}cc@{\hspace{0pt}}c|c@{\hspace{0pt}}cc@{\hspace{0pt}}c|c@{\hspace{0pt}}cc@{\hspace{0pt}}c}}
\bottomrule 
@\grayrow &  @\multicolumn{12}{c}{\textbf{Target}}\\
% &@\multicolumn{10}{c}{\textbf{VOC  \textrightarrow \,  Clipart}} \\  
\toprule
@\textbf{Method} &  @\multicolumn{4}{c}{\textbf{Clipart}} & @\multicolumn{4}{c}{\textbf{Watercolor}} &@\multicolumn{4}{c}{\textbf{Comic}}\\
 &  @AP& & @AP50& & @AP& & @AP50 && @AP& & @AP50 &\\
\midrule
@Faster-RCNN \cite{ren2015faster}  &12.5&&24.1&&19.8&&41.2&&@8.0&&17.9& \\
@RegionCLIP \cite{zhong2022regionclip} &  @16.0&&33.3&&15.9&&44.7&&15.9&&34.2& \\
\cmidrule{1-13}
% @Adaptive MT (CVPR'22) & 17.28 (-2.04)& 40.5 (4.15) & 10.94 (-4.98) & 22.18 & & \\
@Adaptive MT \cite{li2022cross} (CVPR'22) &  14.8&&30.5&&19.9&&43.7&&11.5&&23.4&\\
% @Ours  & 23.05 (+3.73) & 49.56 (+4.91) & 21.66 (+5.74) & 45.87 (+11.65)&& \\
@IRG \cite{vs2022instance} (CVPR'23)&  @-&&31.5&&@-&&@\textbf{53.0}&&@-&&@-& \\
\hline
 @DVA & 17.6&&36.6&&20.1&&43.9&&16.5&&35.9&\\
 @Caption-PL &15.8&&35.2&&20.4&&44.2&&15.6&&34.2&\\
\bfseries @Ours & @\bfseries18.9&&@\bfseries40.4&&@\bfseries22.3&
&49.7&&@\bfseries21.9&&@\bfseries46.3&\\
\bottomrule
 \end{spreadtab}
\end{table}

\begin{table}[!tp]\centering

\scriptsize
\captionsetup{skip=0pt, position=above} % Force the caption to be above the table

\caption{\textbf{Domain Generalization on adverse weather.} City, Foggy \textrightarrow \, Bdd  in $\%$}
\label{tab:DG-city}
\begin{tabular}{l|cccccccc|c}\toprule
\textbf{Method}  &\textbf{prsn} &\textbf{rider} &\textbf{car} &\textbf{truck} &\textbf{bus} &\textbf{train} &\textbf{motor} 
&\textbf{bike} & \textbf{mAP} \\
\toprule

Faster-RCNN \cite{ren2015faster} & 27.9& 27.5& 43.1& 16.6& 15.1& -&5.6 &21.0 &19.6\\
\multirow{8}{*}{}RegionCLIP \cite{zhong2022regionclip}& 40.6& 31.3& 47.9& 16.8 & 12.0&- &11.2 &23.2 &26.1 \\
\cmidrule{1-10}
 DIDN \cite{lin2021domain} (ICCV'21)  &34.5 &30.4 &44.2 &\textbf{21.2} &1\textbf{9.0}&-&9.2 &22.8 & 22.7 \\

Ours  & \textbf{41.4} & \textbf{31.7} & \textbf{49.8} & 18.1& 11.4& -& \textbf{12.4}& \textbf{25.6}&\textbf{27.1} \tiny{\textcolor{blue}{(+7.5)}}\\
\bottomrule
\end{tabular}
\end{table}

\textbf{Adverse weather.}
Similarly, Faster-RCNN and RegionCLIP trained on City are considered source-only FSOD baselines in both DG and DA tasks. Table \ref{tab:DG-city} illustrates the superiority of our method compared to the baselines and DIDN on \textit{City, Foggy $\rightarrow$ Bdd} generalization task. Our methods outperform DIDN by a large margin, despite DIDN's significantly more complex training process. Specifically, DIDN requires a domain-invariant encoder and decoder to be trained along with a domain-specific encoder for each source domain at both the image-level and instance-level. This adds significant computation overhead, especially when the number of source domains (i.e., $K$ in the main text) is large. On the other hand, our method requires a single $v2l$ layer which is shared between all source domains during the training. In Table 2 in the main text, we extensively compared our method on \textit{City $\rightarrow$ Foggy} adaptation task. Please refer to the main text for more information.

\textbf{Stability comparison.} Fig. \ref{fig:delta_comparison} demonstrates the stability of our method compared to the domain adaptation methods on the real-to-artistic benchmark. We define $\Delta = DA_{mAP} - DG_{mAP}$. For example, for Clipart, we subtract the average performance on Clipart when Clipart is used as a target domain in DG task (i.e., Table \ref{tab:DG-voc-supplement}) from the performance on Clipart in a DA task (i.e., Table \ref{tab:DA-voc}). Our model mAP drop on DG sets is relatively much lower than the DA methods, especially on Clipart and Watercolor. For example, on Clipart, our model's performance drops by 1.15\%, while Adaptive-MT-RN50's performance drops  by 3.15\% and Adaptive-MT-RN101's performance drops by 4.8\%. While comic $\Delta$ for our model is higher than Adaptive-MT-RN50, this is due to the fact that Adaptive-MT-RN50 performs poorly on Comic in both DA and DG settings. For instance, in DA task, our model achieves 46.3\% while Adaptive-MT-RN50 achieves 23.4\% (Table \ref{tab:DA-voc}), and the average performance in the DG settings is 45.2\% and 23.25\% for ours and Adaptive-MT-RN50, respectively (see Table \ref{tab:DG-voc-supplement}).

\begin{figure}
    \centering
    \includegraphics[width=0.6\textwidth]{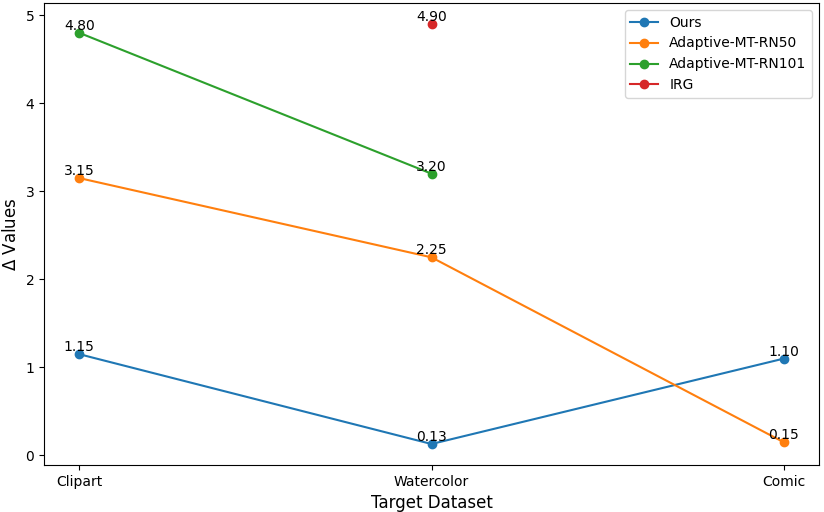} % Replace with the actual filename and path
    \caption{\textbf{Comparison of $\Delta$}. $\Delta$ represents the drop in the performance on the target, when the target is used as the source domain (i.e. DA) and when it is unknown throughout the training (i.e. DG). Hence, a lower number means that the model is more stable. Adaptive-MT-RN101 and IRG values are borrowed from \cite{li2022cross} and \cite{vs2022instance}, respectively. Since values for all settings were not reported, $\Delta$ is reported in Clipart and Watercolor for Adaptive-MT-RN101 and in Watercolor for IRG. RN101 is the ResNet101 backbone, while RN50 is the ResNet50 backbone. }
    \label{fig:delta_comparison}
\end{figure}

\section{Qualitative results \& examples}

\textbf{Caption comparison.} Table \ref{tab:caption-compare} includes some examples of the generated caption on the validation set of VOC, Clipart, Watercolor, and Comic. Specifically, we use ClipCap to generate captions based on RegionCLIP baseline trained on VOC in a supervised manner and when our method is trained on \textit{VOC, Clipart $\rightarrow$ Watercolor, Comic}. Even though our method does not produce a perfect caption, especially in artistic domains, it constantly produces better and more meaningful captions than the RegionCLIP baseline. Captions may become meaningless on natural images from the VOC dataset when representation is trained for object detection. For instance, in Table \ref{tab:caption-compare} RegionCLIP baseline generated an unrelated caption for the image from the VOC dataset that is missing the essential information such as "A person" and a "horse". This shows the importance of our proposed knowledge distillation based regularization technique to ensure that captions are meaningful and related to the corresponding image.  

\begin{table}[!tp]
\scriptsize
\centering
\captionsetup{skip=0pt, position=above} % Force the caption to be above the table
\caption{\textbf{Caption Comparison}. Comparing generated caption based on RegionCLIP baseline and CDDMSL visual features when training using VOC and Clipart as source domains }
\label{tab:caption-compare}
\begin{tabular}{@{\hspace{0pt}}l@{\hspace{2pt}}c@{\hspace{0pt}}c@{\hspace{0pt}}c@{\hspace{0pt}}c@{\hspace{0pt}}}
% \hline
 & VOC &Clipart&Watercolor&Comic\\ 

& \includegraphics[width=0.115\textwidth]{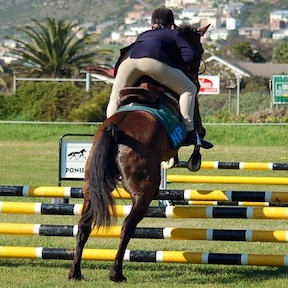} &
\includegraphics[width=0.115\textwidth]{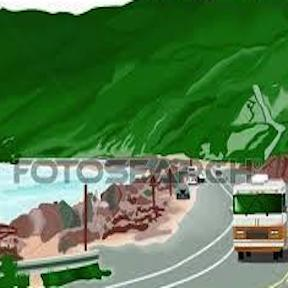} & 
\includegraphics[width=0.12\textwidth]{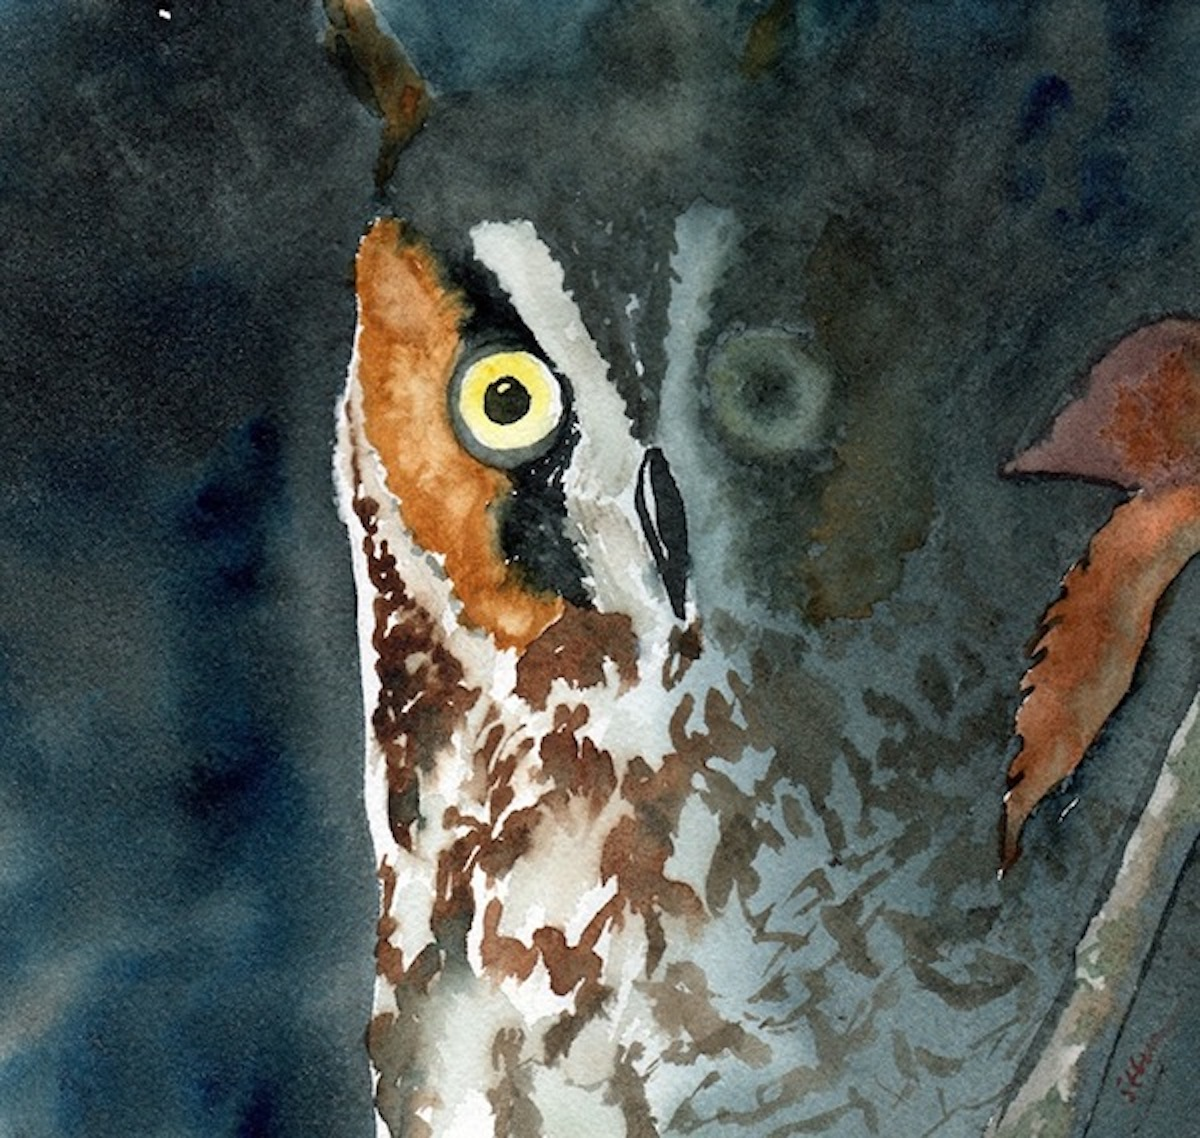} & 
\includegraphics[width=0.115\textwidth]{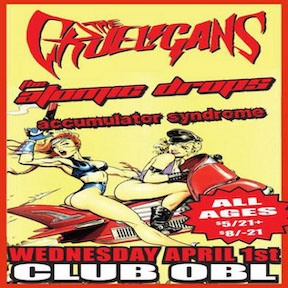} \\

RegionCLIP & \multicolumn{1}{p{1.7cm}}{\raggedright Two people are standing in a room with a table.} & \multicolumn{1}{p{1.7cm}}{\raggedright A row of soccer jerseys on a rooftop} &
\multicolumn{1}{p{1.7cm}}{\raggedright A picture of a wall of knit hats} & \multicolumn{1}{p{1.9cm}}{\raggedright A man is standing in a coffee shop with a group of people watching him.} \\ \hline

Ours &\multicolumn{1}{p{1.7cm}}{\raggedright A person riding a brown horse on a paved field.} &  \multicolumn{1}{p{1.7cm}}{\raggedright A green and white truck driving down a beach.} &
\multicolumn{1}{p{1.7cm}}{\raggedright A brown and white drawing of a bird.} & 
\multicolumn{1}{p{1.7cm}}{\raggedright A man riding a motorcycle on top of a building}\\ \hline
\end{tabular}

\end{table}

% \begin{table}[!tp]
% \scriptsize
% \centering
% \captionsetup{skip=0pt, position=above} % Force the caption to be above the table
% \caption{Visualization inference of our model on real-to-artistic and adverse-weather domains. RegionCLIP (top) is trained on labeled data. Ours (bottom) is trained on VOC and Clipart for real-to-artistic generalization and City and Foggy for adverse-weather generalization. }
% \label{tab:predictions-compare}
% \begin{tabular}{@{\hspace{0pt}}l@{\hspace{2pt}}c@{\hspace{0pt}}c@{\hspace{0pt}}c@{\hspace{0pt}}c@{\hspace{0pt}}}
% % \hline

% \raisebox{1.5cm}{\textbf{R-CLIP}}& \includegraphics[width=0.2\textwidth]{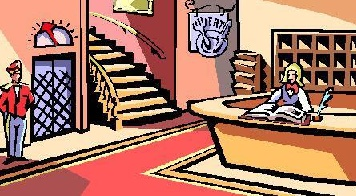} &
% \includegraphics[width=0.2\textwidth]{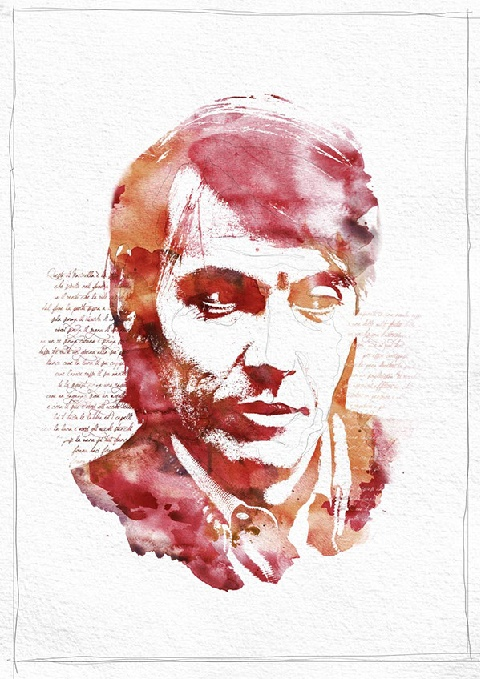} & 
% \includegraphics[width=0.2\textwidth]{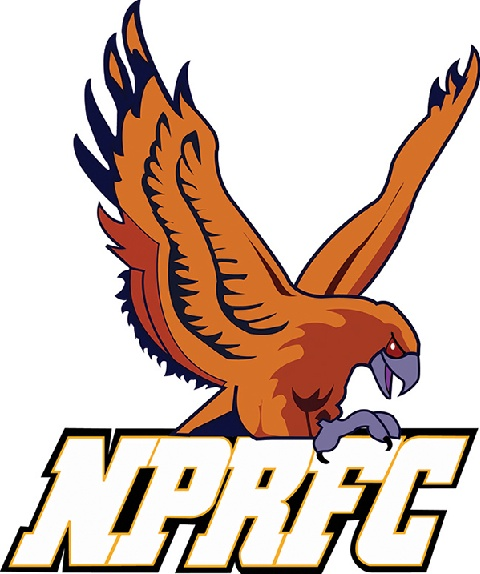} & \includegraphics[width=0.2\textwidth]{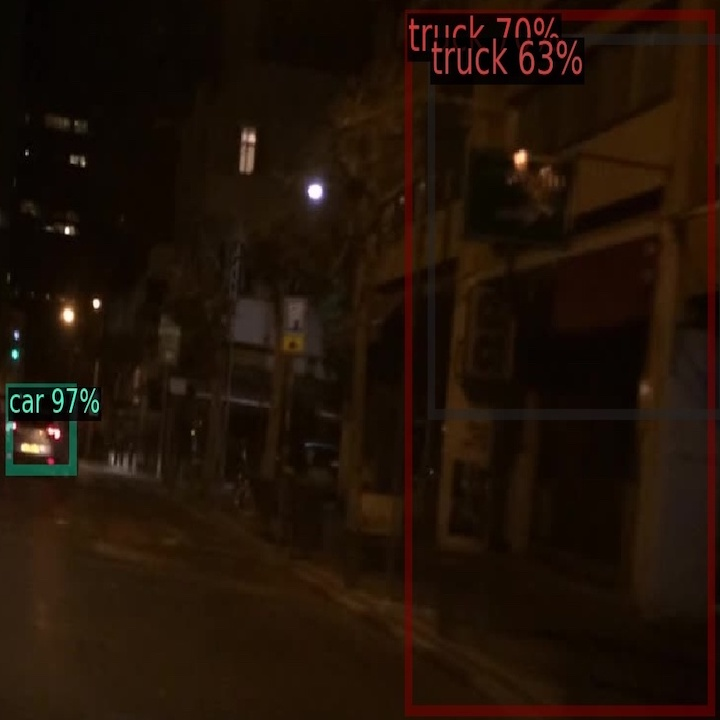}
%  \\ 
    
%     \raisebox{1.5cm}{\textbf{Ours}} & \includegraphics[width=0.2\textwidth]{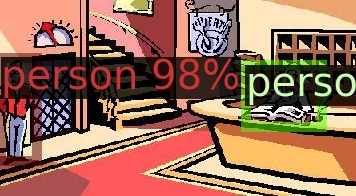} &
% \includegraphics[width=0.2\textwidth]{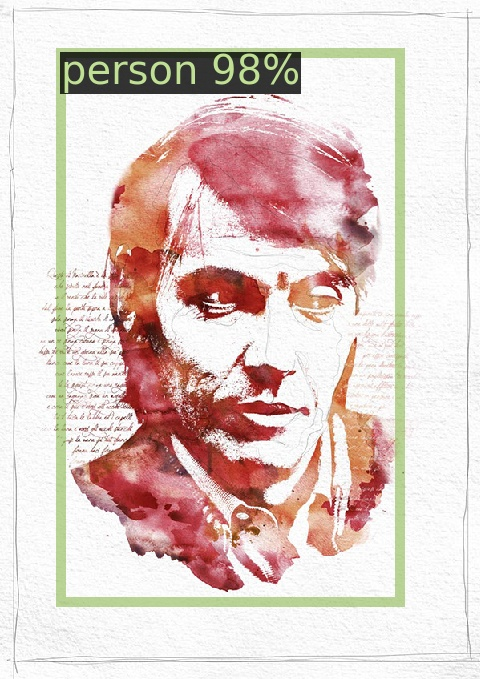} & 
% \includegraphics[width=0.2\textwidth]{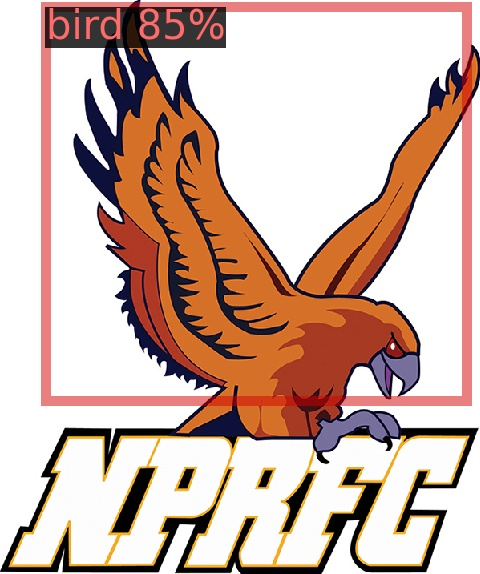} &   \includegraphics[width=0.2\textwidth]{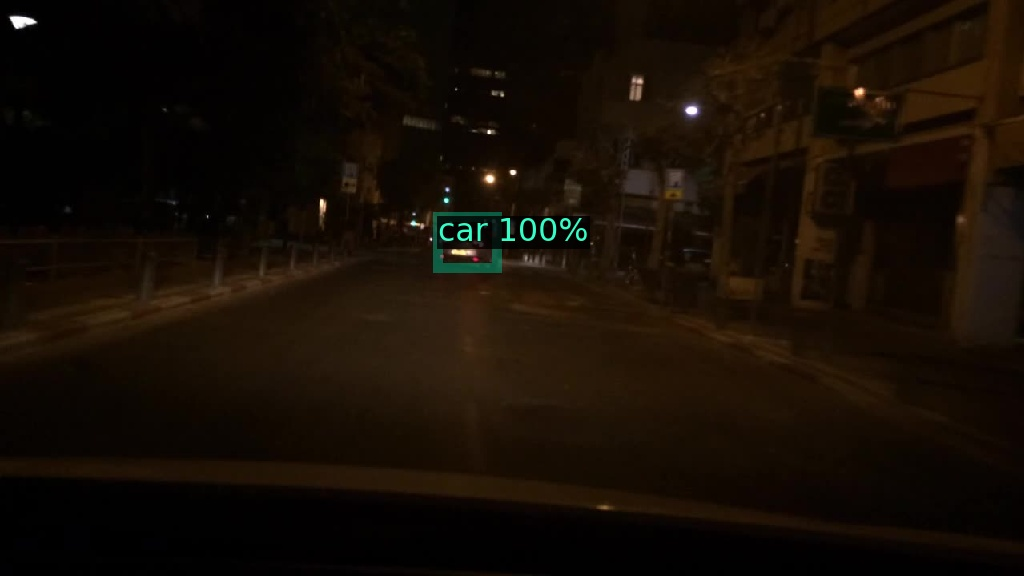}\\ 
% & Clipart & Watercolor & Comic & Bdd

% \end{tabular}

% \end{table}

\begin{table}[!tp]
\scriptsize
\centering
\captionsetup{skip=0pt, position=above} % Force the caption to be above the table
\caption{Visualization inference of our model on real-to-artistic. Each pair of columns corresponds to a different sample with RegionCLIP (left column in each pair) trained on labeled data and Ours (right column in each pair) trained on VOC (labeled) and Clipart (unlabeled) for real-to-artistic generalization.}
\label{tab:predictions-compare-voc}

\begin{tabular}{l@{\hspace{2pt}}c@{\hspace{2pt}}c@{\hspace{2pt}}|@{\hspace{2pt}}c@{\hspace{2pt}}c}
% \hline
\raisebox{1.5cm}{\textbf{Clipart}} &\includegraphics[width=0.2\textwidth,height=0.2\textwidth]{images/pred_comp/real-to-artistic/clipart/baseline/img_201800020.jpg} &
\includegraphics[width=0.2\textwidth,height=0.2\textwidth]{images/pred_comp/real-to-artistic/clipart/ours/img_201800020.jpg} & \includegraphics[width=0.2\textwidth,height=0.2\textwidth]{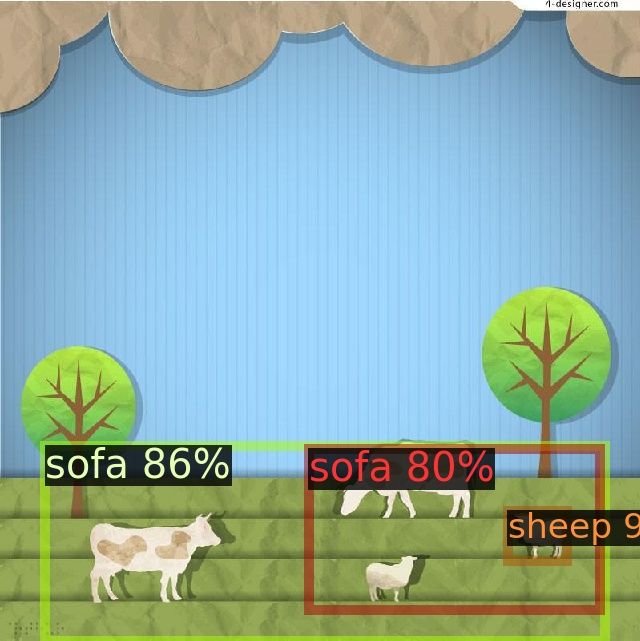} &
\includegraphics[width=0.2\textwidth,height=0.2\textwidth]{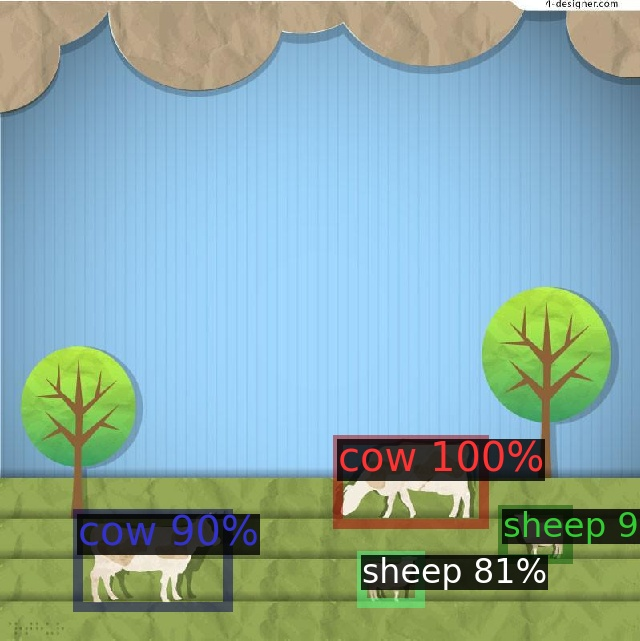} \\

\raisebox{1.5cm}{\textbf{Watercolor}} & \includegraphics[width=0.2\textwidth,height=0.2\textwidth]{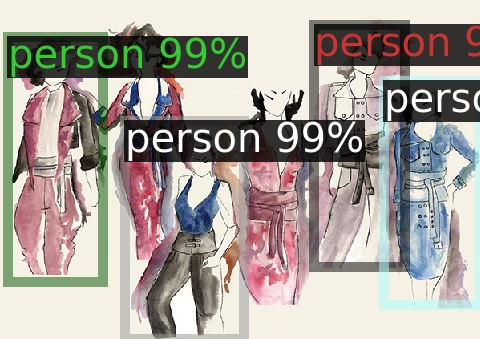} &
\includegraphics[width=0.2\textwidth,height=0.2\textwidth]{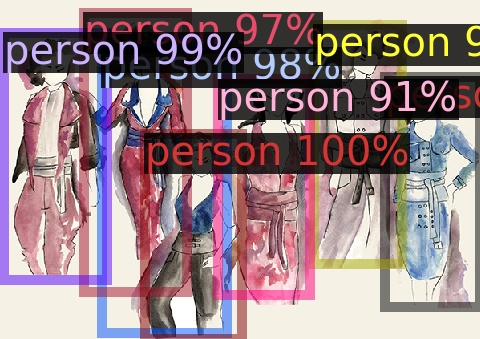}
& \includegraphics[width=0.2\textwidth,height=0.2\textwidth]{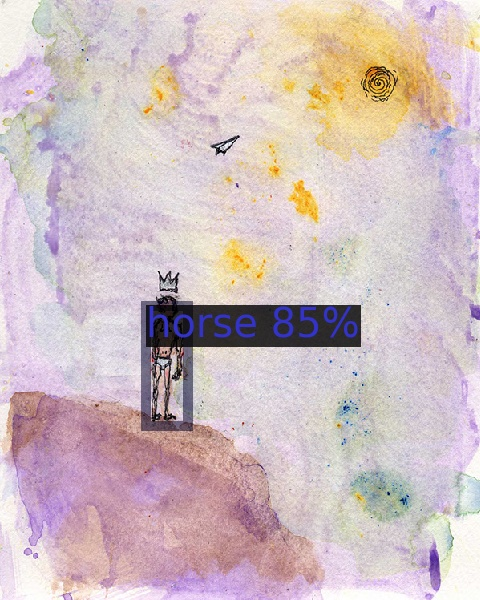} &
\includegraphics[width=0.2\textwidth,height=0.2\textwidth]{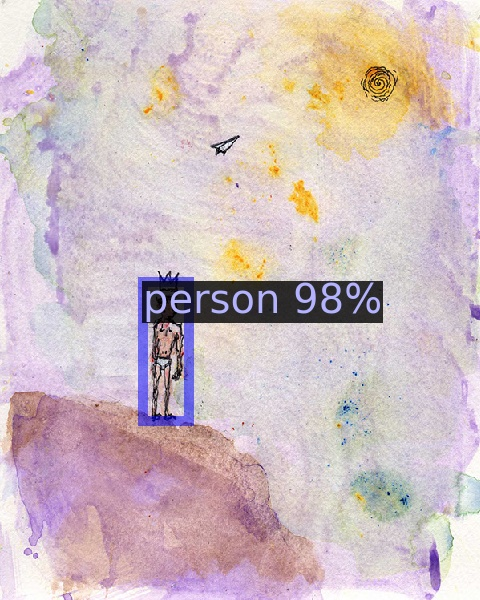}\\

 \raisebox{1.5cm}{\textbf{Comic}} & \includegraphics[width=0.2\textwidth,height=0.2\textwidth]{images/pred_comp/real-to-artistic/comic/baseline/img_33497847.jpg} & 
\includegraphics[width=0.2\textwidth,height=0.2\textwidth]{images/pred_comp/real-to-artistic/comic/ours/img_33497847.jpg}  
&\includegraphics[width=0.2\textwidth,height=0.2\textwidth]{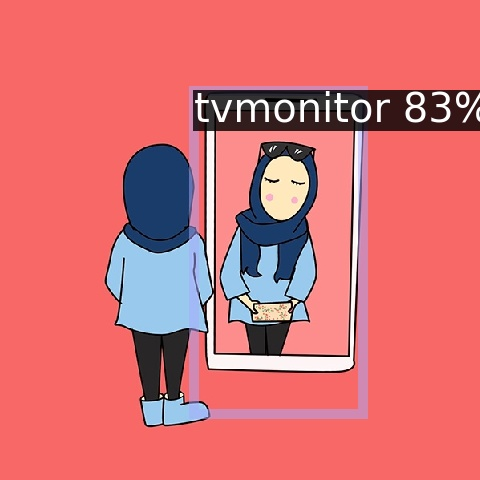} & 
\includegraphics[width=0.2\textwidth,height=0.2\textwidth]{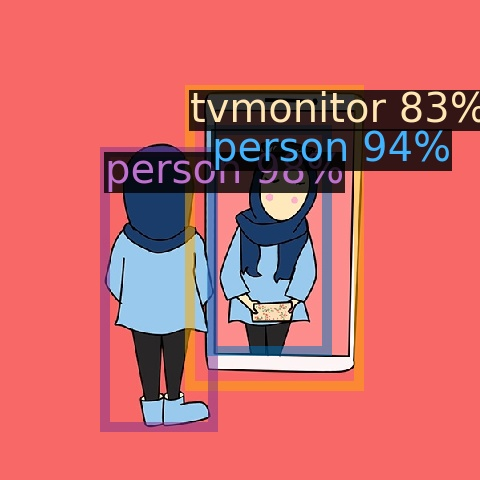}  \\
& \textbf{R-CLIP} & \textbf{Ours}& \textbf{R-CLIP} & \textbf{Ours}\\
\end{tabular}
\end{table}

\begin{table}[!tp]
\scriptsize
\centering
\captionsetup{skip=0pt, position=above} % Force the caption to be above the table
\caption{Visualization inference of our model on adverse-weather domains. RegionCLIP (left column) is trained on labeled data. Ours (right column) is trained on City and Foggy for adverse-weather generalization. The first two rows are results from Foggy, and the last three rows are predictions on the Bdd test set.}
\label{tab:predictions-compare-city}
\begin{tabular}{l@{\hspace{2pt}}c@{\hspace{2pt}}c@{\hspace{2pt}}}
& \includegraphics[width=0.5\textwidth]{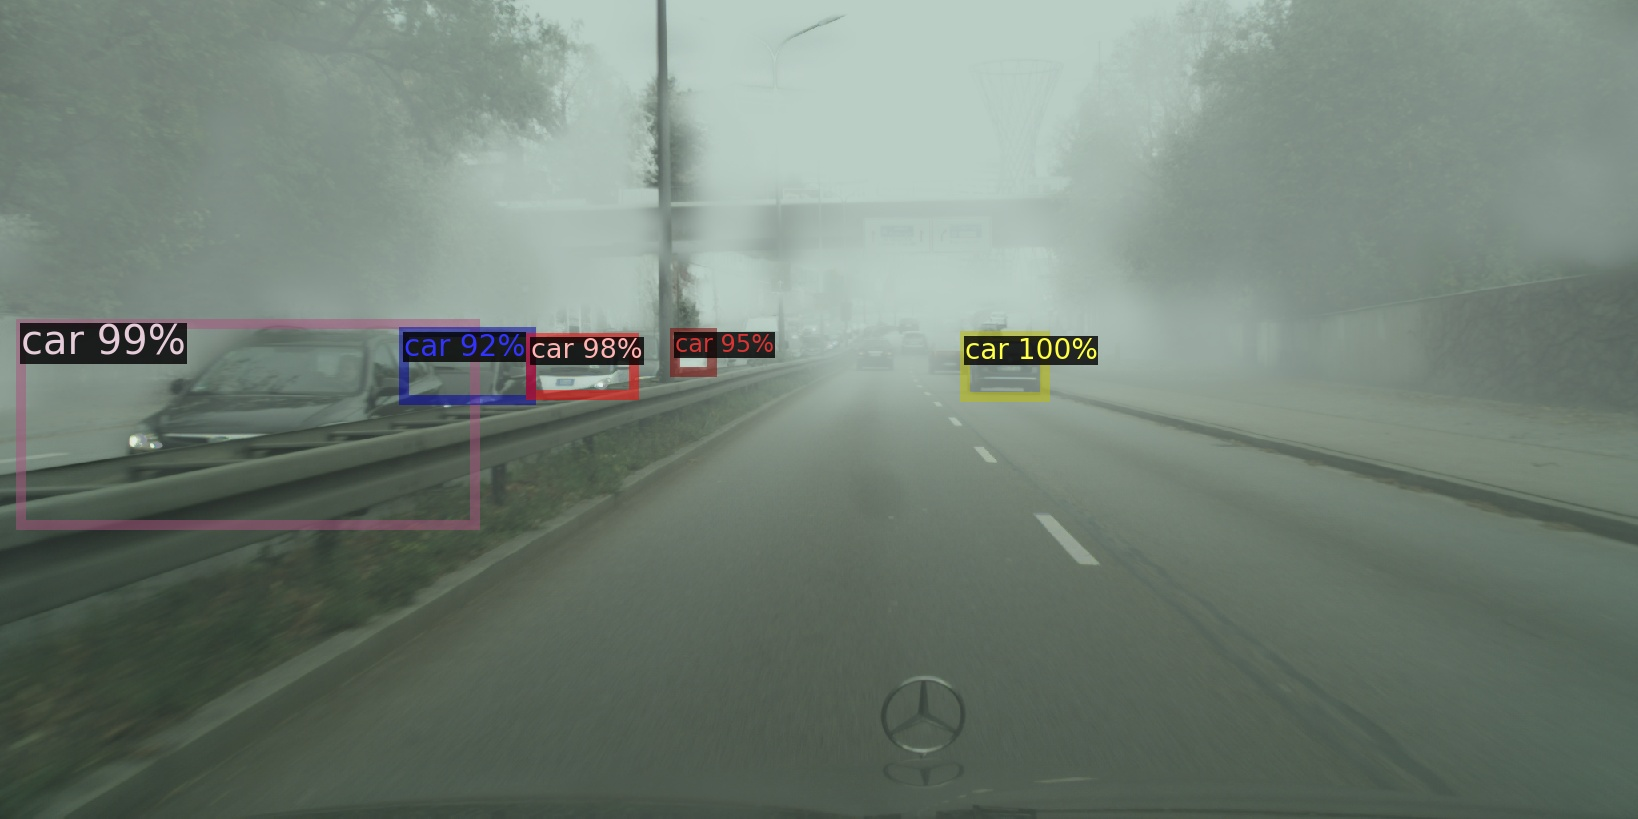} &
\includegraphics[width=0.5\textwidth,]{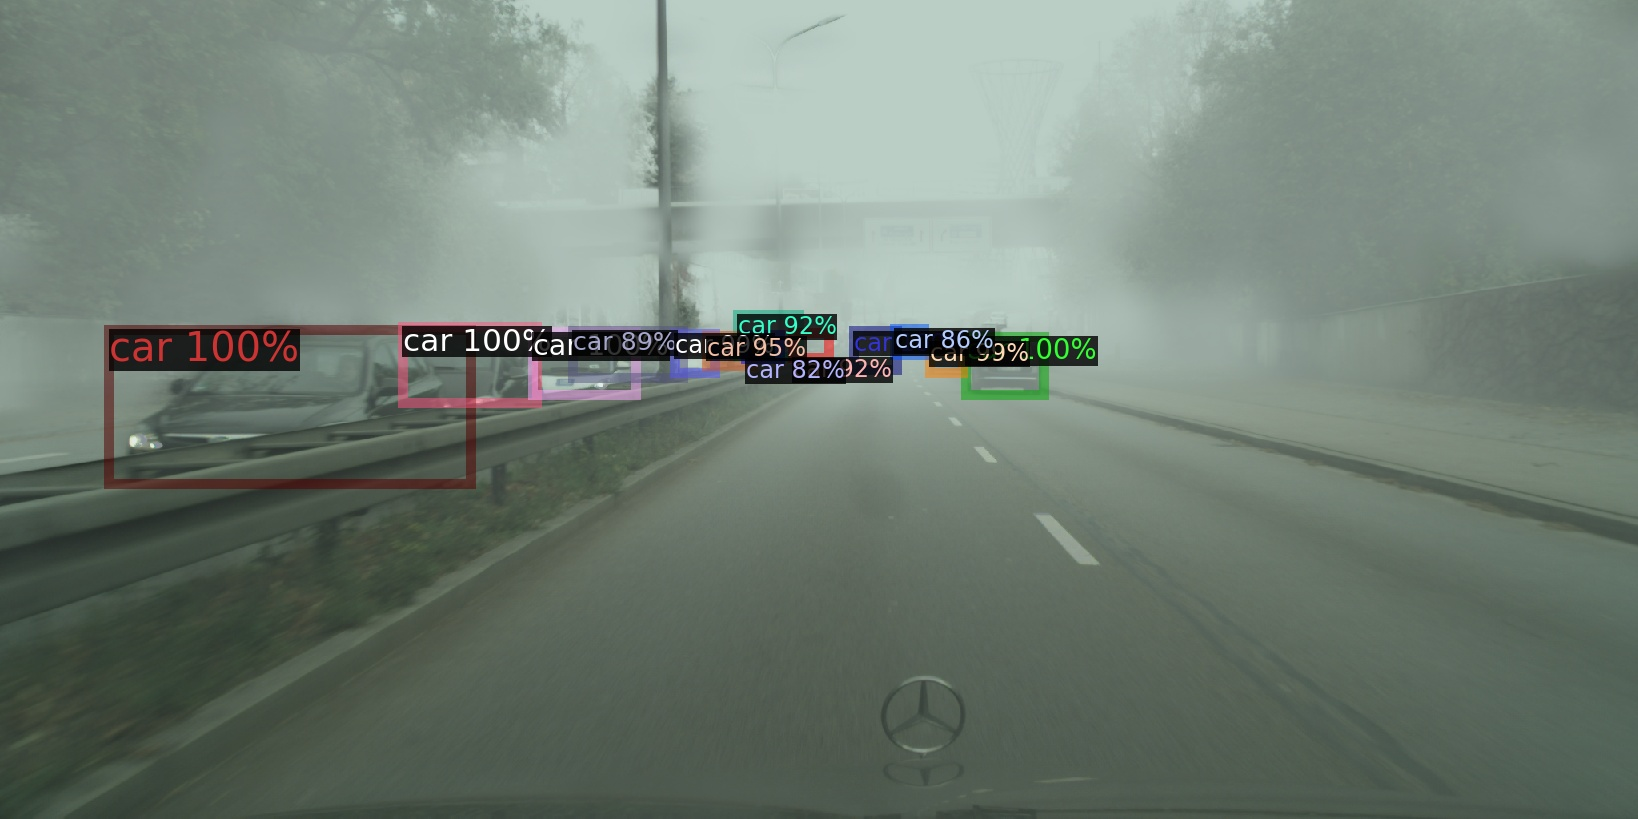} \\

& \includegraphics[width=0.5\textwidth]{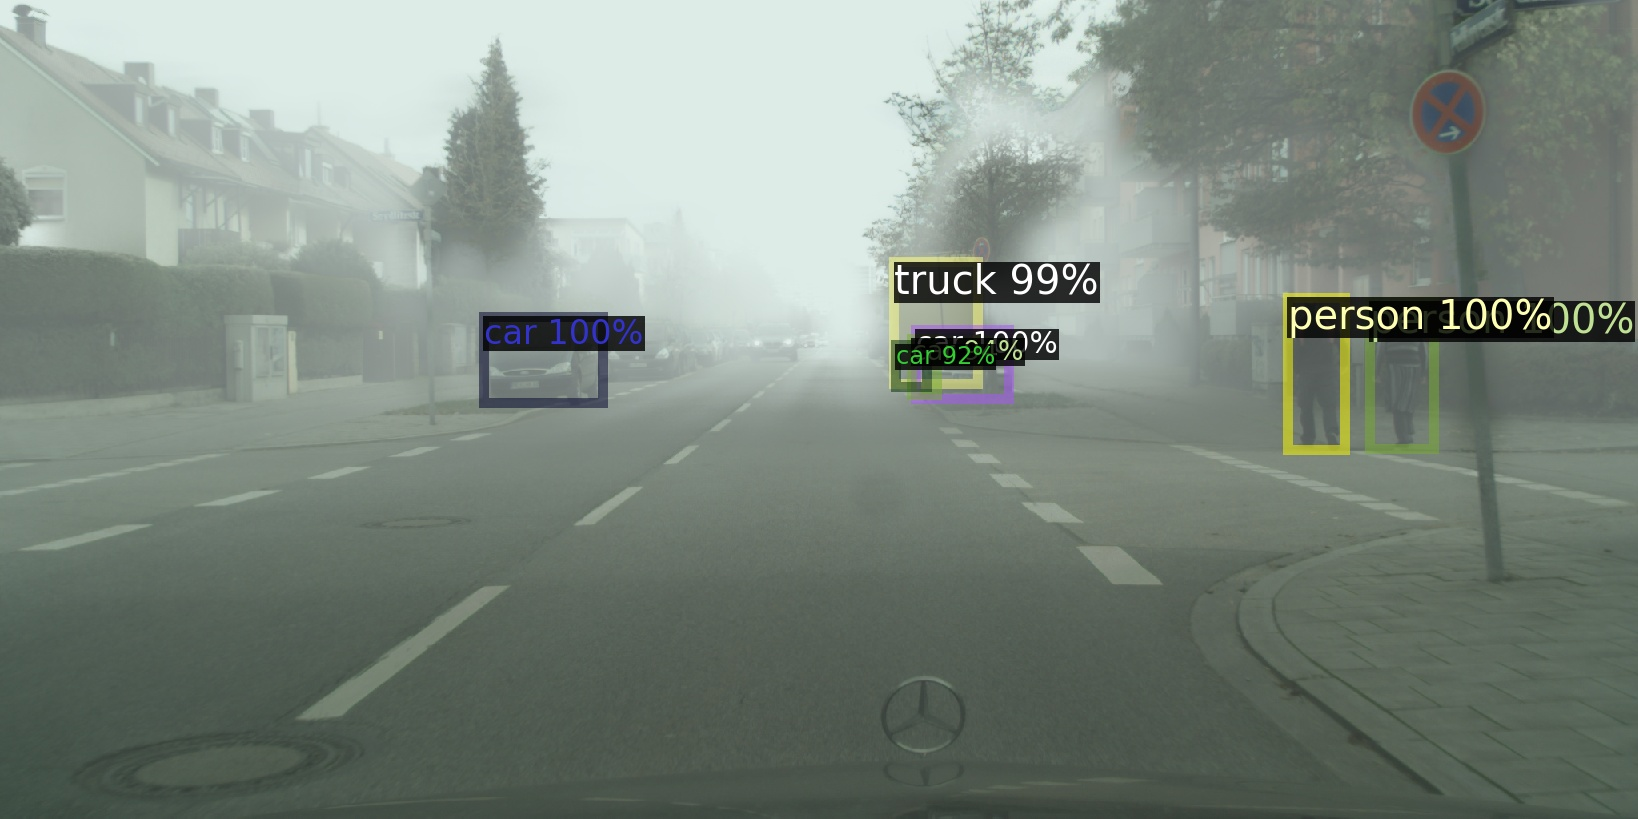} &
\includegraphics[width=0.5\textwidth,]{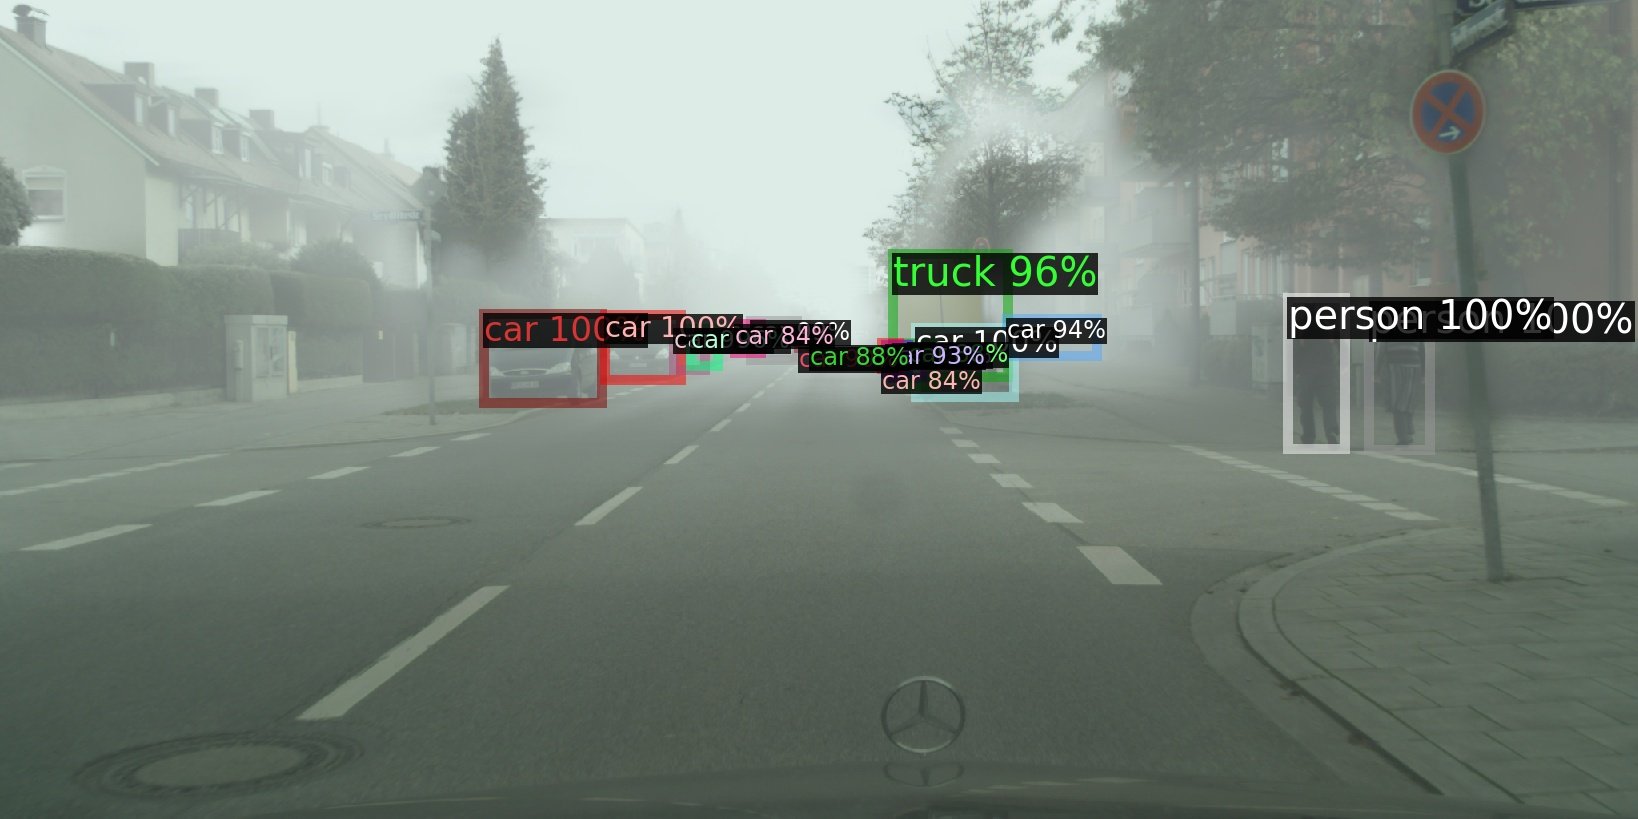} \\

\midrule
& \includegraphics[width=0.5\textwidth]{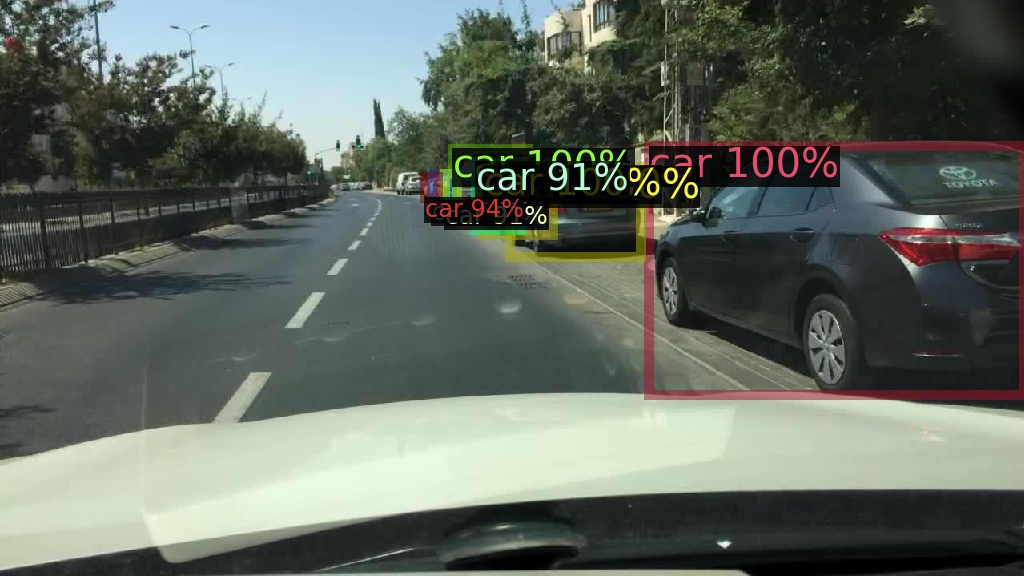} &
\includegraphics[width=0.5\textwidth,]{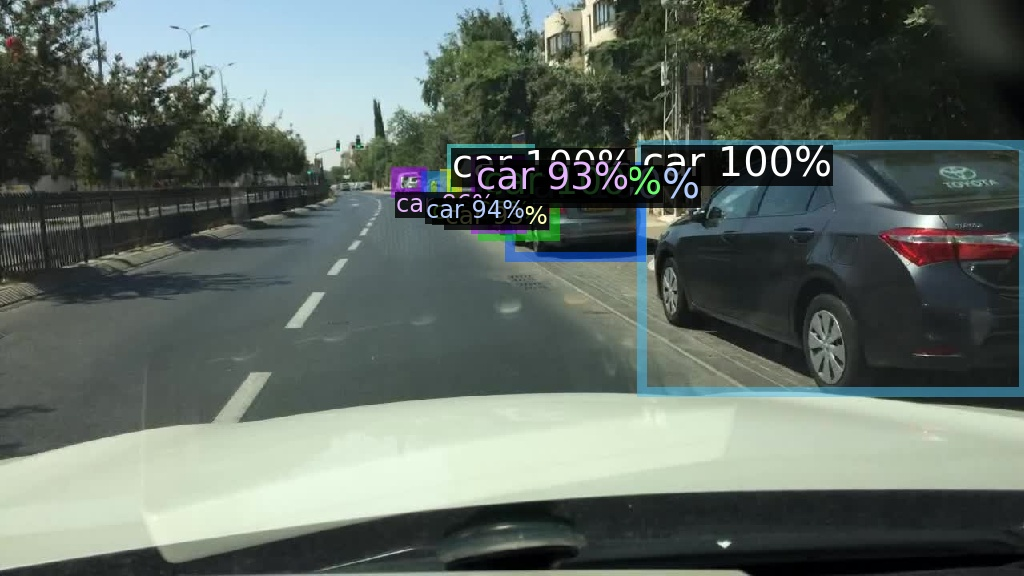} \\

& \includegraphics[width=0.5\textwidth]{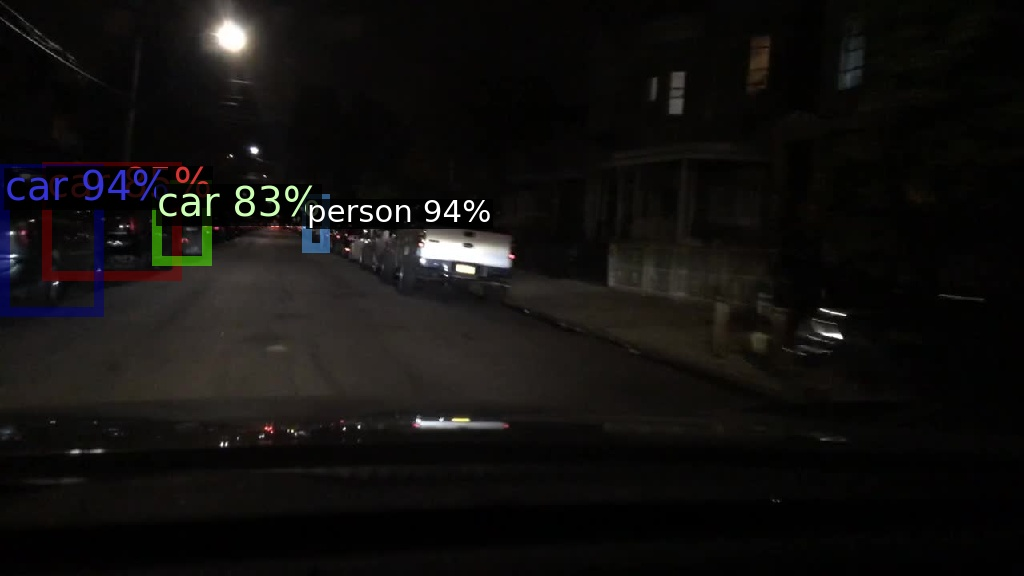} &
\includegraphics[width=0.5\textwidth,]{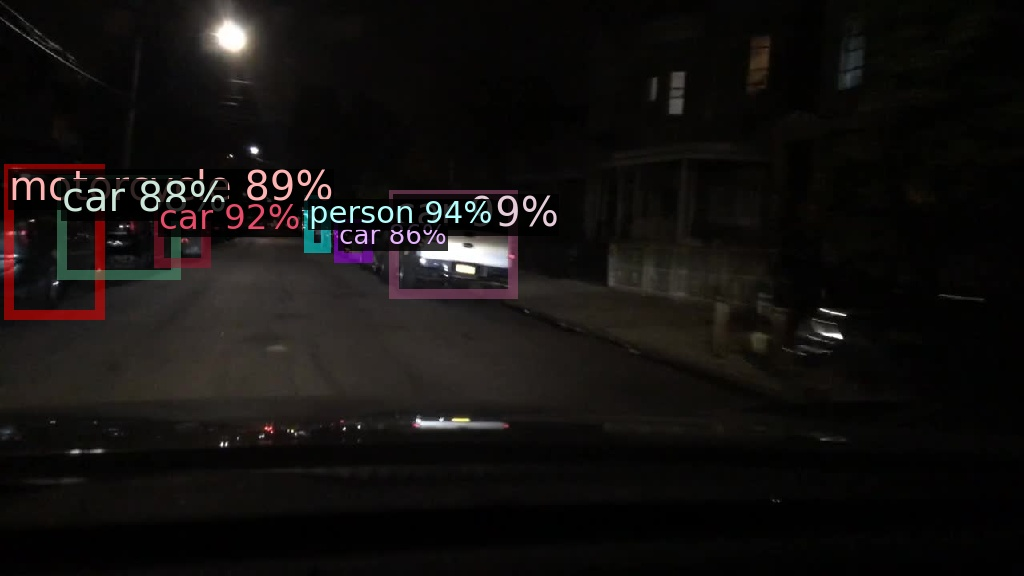} \\

& \includegraphics[width=0.5\textwidth]{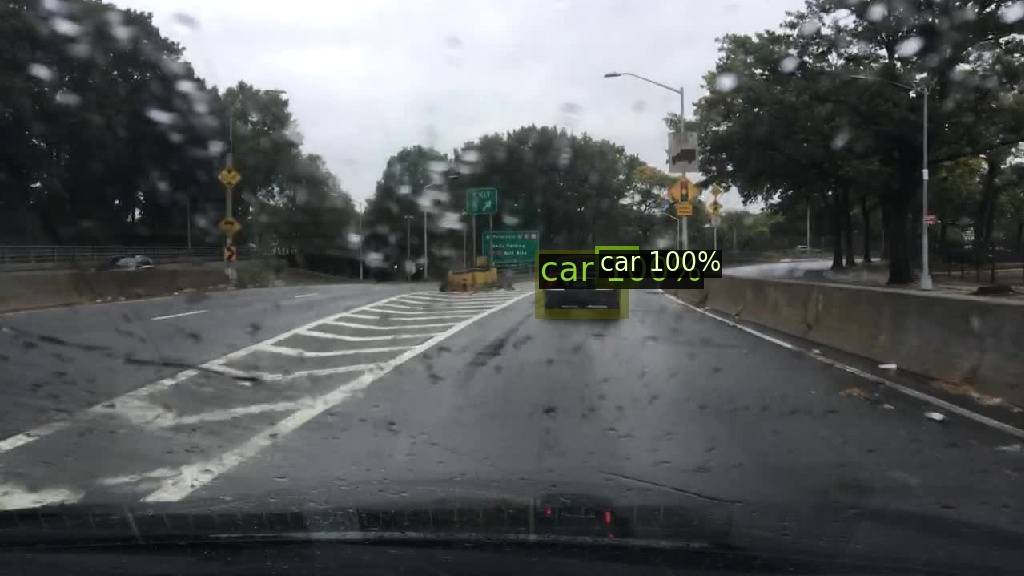} &
\includegraphics[width=0.5\textwidth,]{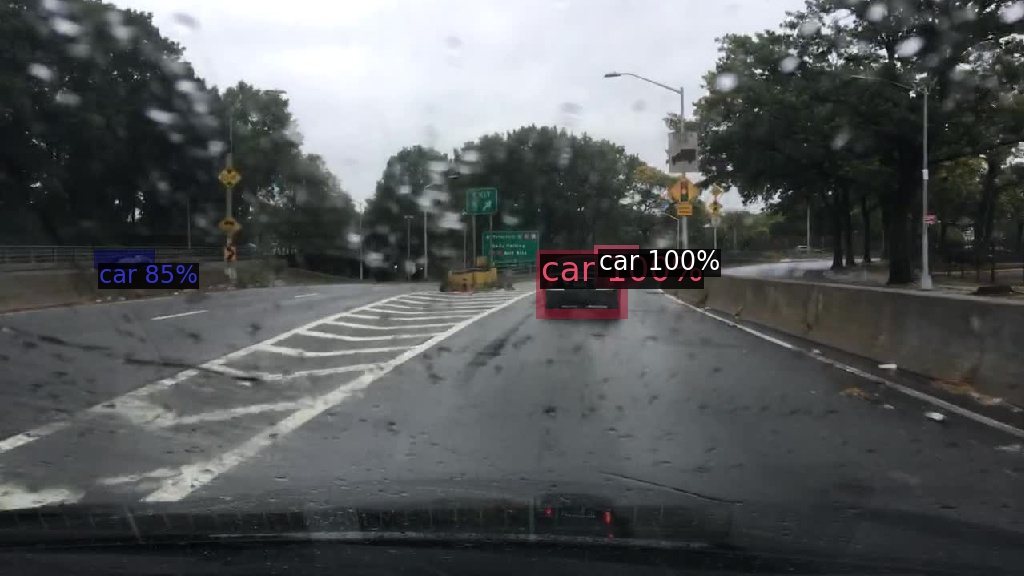} \\

& \textbf{R-CLIP} & \textbf{Ours}\\
\end{tabular}
\end{table}

% \begin{tabl

% ********** PLEASE READ COMMENT **********

% I think we can use the following if reviewers ask questions or raise any concerns about the baselines:

% (\textbf{comment: I think we can comment the following here and use it if reviewers ask questions or raised any concerns about the baselines: }It is worth mentioning that unsupervised domain adaptation works can be extended for DGOD and SSDG problems. In fact, Adaptive-MT is the only model reporting their result on DGOD on this task. Therefore, we also compared our model against recent DA methods and showed the advantage of CDDMSL on DG and SSDG. 
